# Supplementary material for: Force-induced Catastrophes on Energy Landscapes: Mechanochemical Manipulation of Downhill and Uphill Bifurcations Explains Ring-opening Selectivity of Cyclopropanes
Source: arXiv:2103.15517 ancillary file (2021-03-29)
Supplement: Supplementary file 1 [file SI.pdf]

# 1 Cyclopropane Derivatives

## 1.1 Nomenclature of Reactant and Product States

In the main text, we often use shorthand notations for the reactant as well as for the products of the ring-opening reaction for simplicity. The reactant species that we investigated previously [1,2] and also here, namely (2$S$,3$S$)-1,1-dichloro-2,3-dimethylcyclopropane according to IUPAC nomenclature, is also denoted by *trans*-1,1-dichloro-2,3-dimethylcyclopropane or *trans*-*gem*-dichlorocyclopropane or *trans*-*g*DCC in the literature. The corresponding difluoro, dibromo and diiodo derivatives can be denoted analogously. For the products, we chose a nomenclature based on the con- or disrotatory opening of the ring together with the direction of the halogen migration to the left or right side with respect to our reference frame as depicted for the chloro derivative in Fig. S1. Upon ring-opening and subsequent halogen migration, the so-called dis-left, dis-right, con-left and con-right product states can be reached. First, the direction of the rotation of the right methyl group (carbon atom C5) leads to the distinction in disrotatory (dis) and conrotatory (con) paths and thus products. Second, the chlorine atom Cl7 may migrate either to what we call here the "left" carbon C2 or the "right" carbon C4 according to the specific (albeit arbitrary) reference frame provided in Fig. S1.

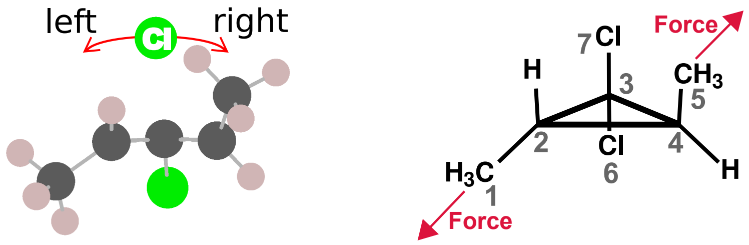


a) Left/right migration    b) Atom numbering

Figure S1: Reference frame used to introduce our shorthand nomenclature of the ring-opening products.

The systematic nomenclature of the reactant and the four product states for the dichloro derivative according to IUPAC reads as follows:

- *trans*-*g*DCC reactant = (2$S$,3$S$)-1,1-dichloro-2,3-dimethylcyclopropane
- dis-left product = ($E$)-(4$S$)-3,4-dichloro-2-pentene
- dis-right product = ($Z$)-(4$S$)-3,4-dichloro-2-pentene
- con-left product = ($Z$)-(4$S$)-3,4-dichloro-2-pentene
- con-right product = ($Z$)-(4$R$)-3,4-dichloro-2-pentene

The corresponding difluoro, dibromo and diiodo derivatives that we investigated in the thermal limit can be denoted analogously.

The dis-right and con-left products posses the same IUPAC name and indeed, at a first glance, one could question the discrimination that we introduce here. But there are two good reasons to treat them differently. First, they differ in the rotation of the substituents at the quaternary carbon atom which is not covered

in the usual IUPAC nomenclature because rotations around such carbon-carbon single bonds possess low energy barriers. Second, being the main argument, the two structures arise here from two totally different reaction pathways, namely one being a disrotatory ring-opening while in the other the methyl groups both turn outward in a conrotatory fashion.

## 1.2 Thermal Reactions of *trans-g*DFC

It is well established theoretically [3] as well as experimentally [4,5] that the thermal reaction of *trans-g*DFC prefers to proceed *via* disrotatory ring-opening and closing pathways as depicted schematically in the upper part of Fig. S2. Ring-opening followed by fluorine migration as investigated in this study and shown in the lower part of Fig. S2, however, has not been reported up to now although it is the preferred reaction for *trans-g*DCC as supported by theory [1,2] and experiment [6,7]. In order to systematically understand how bifurcations can be tuned by means of chemical substitution, we were able to optimize the transition states (TSs) of the disrotatory ring-opening followed by fluorine migration for *trans-g*DFC as presented in the main text as well as in the following sections of the SI using density functional theory as detailed below. We show in this section that these are energetically higher-lying reaction channels compared to the established pathways. [3,4]

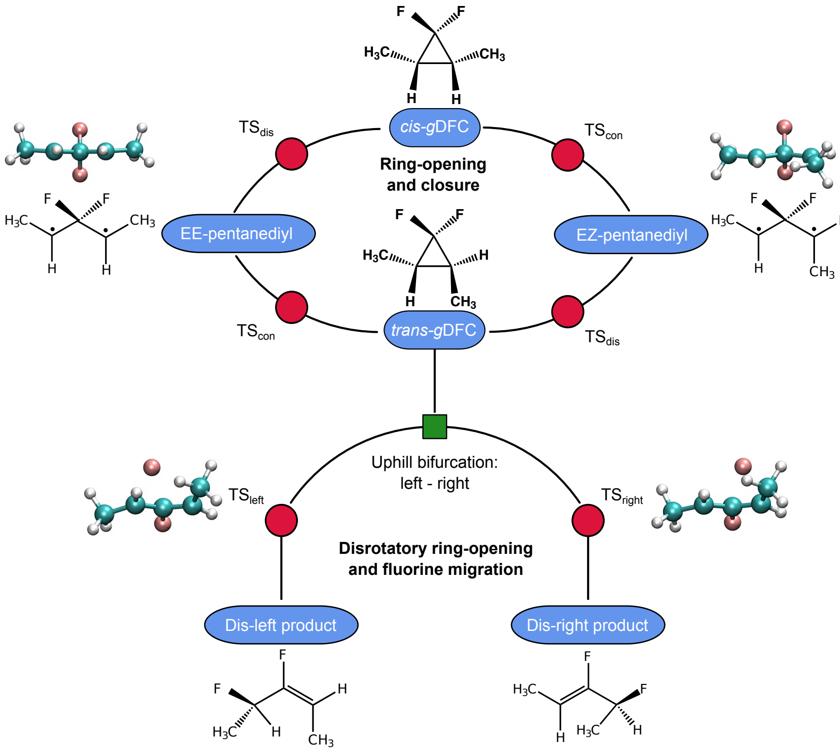


Figure S2: Reaction scheme of (2*S*,3*S*)-1,1-difluoro-2,3-dimethylcyclopropane in the thermal reference case. The upper cycle shows the preferred [3,4] ring-opening and closing reactions, while the lower part depicts the disrotatory ring-opening reaction in combination with fluorine migration. Reactant and product minima, transition states, and bifurcations are depicted in blue, red and green, respectively.

Since the previously reported ring-opening and closing pathways [3,4] feature diradical intermediates, we applied multi-reference methods, in particular CASSCF(4,4)

with the def2-TZVP basis set, for the optimization of reactant and transition state structures, followed by adding the NEVPT2 single-point correction (using the same basis set) to account for dynamical electron correlation effects. These calculations have been performed with the ORCA program package. [8] With this accurate description of the electronic structure we are able to optimize the same TSs as obtained from density functional theory, see below. In addition, the reactant *trans-g*DFC and the planar E,E-(0,0) and E,Z,-(0,0) 3,3-difluoropentane-l,3-diyles (minimia on the potential energy surface (PES), abbreviated as EE-pentanediyle and EZ-pentanediyle in Fig. S2) were optimized.

Overall this yields the following energetic ordering: The singlet diradicals E,E-(0,0) and E,Z,-(0,0) 3,3-difluoropentane-l,3-diyles, as already reported in a pioneering study, [3] lie about 43.9 $\mathrm{kcal\,mol^{-1}}$ and 50.5 $\mathrm{kcal\,mol^{-1}}$ higher in energy than the reactant, while the TSs of the left and right migration are 66.6 $\mathrm{kcal\,mol^{-1}}$ as well as 66.9 $\mathrm{kcal\,mol^{-1}}$ higher in energy, respectively. These results show that disrotatory ring-opening with fluorine left/right migrations, as reported in the main text, follow energetically higher-lying reaction pathways compared to the established reactions, but are of particular interest in the present case to compare to the differently substituted reactants. In the following, we will thus concentrate on these reaction pathways. It is mentioned in passing that fluorine migration subsequent to ring-opening could indeed be an alternative explanation of competing reaction(s) of *cis-g*DFC to *trans-g*DFC isomerization as experimentally observed at higher forces in certain solvents. [5]

## 1.3 Intrinsic Reaction Coordinates and Energy Profiles

Optimization of TSs and the Intrinsic Reaction Coordinates (IRCs) of the four halogen-substituted cyclopropane derivatives have been performed using the unrestricted BLYP density functional and the TZVP basis set as implemented in Gaussian 09 [9]. As before, [2] the IRCs are parameterized in terms of the Root Square Displacements (RSDs) of all heavy atoms. Therefor, the structural change $(\vec{r}_f - \vec{r}_{f-1})$ of these atoms between all adjacent discrete configurations along the generated path is calculated. The TS corresponds to $\vec{r}_0$ and is set to RSD $= 0\,\text{Å}$. The RSD of a specific structure $n$ is evaluated as the accumulation of the geometrical displacements along the IRC starting from the TS up to the desired point. The overall sign of the RSD is chosen such that negative / positive values indicate evolution toward the reactant / product side.

$$\mathrm{RSD}\,(n) = \sum_{f=1}^{n} \left( \sum_{\substack{\text{heavy}\\\text{atoms}}} (\vec{r}_f - \vec{r}_{f-1})^2 \right)^{1/2}$$

Subsequent frequency analyses along the reaction path, see next section, were carried out with the same method and basis set as used for the calculation of the IRCs. Starting from the TS of the symmetry-allowed disrotatory ring-opening for the dichloro derivative at zero force, i.e. upon purely thermal activation, a series of force-transformed TSs has been obtained exclusively for the dichloro derivative by successively increasing the constant force. [2] At forces exceeding 1.6 nN, the mechanism is found to switch from dis- to conrotatory ring-opening, which has been followed up to 3.0 nN. We found previously [2] that the complete set of IRCs of the conrotatory mechanism down to 0.0 nN could be generated upon taking the conrotatory

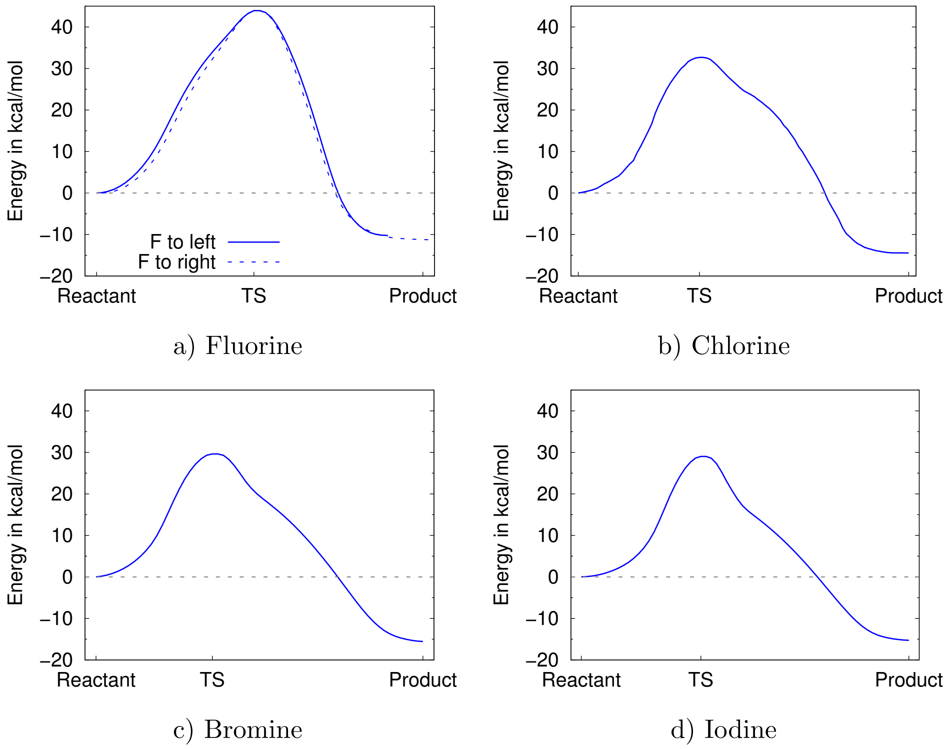


Figure S3: **Energies along the disrotatory IRCs dependent on the substitution of trans-1,1-dihalo-2,3-dimethylcyclopropane in the thermal reference case.** The structures and energies along the IRCs have been obtained with the TZVP basis set and the unrestricted BLYP density functional (with very tight convergence criteria and ultrafine integration grids) as implemented in Gaussian 09 [9].

TS at 1.7 nN, where it becomes preferred over disrotatory ring-opening, and stepwise lowering the applied force. This provides us with the force-dependence of the activation energy corresponding to the conrotatory reaction all the way from 0 nN, where it is symmetry-forbidden, up to 3 nN as shown in the SI of Ref. 2.

The energies along the IRCs for disrotatory ring-opening in the thermal reference limit are reported in Fig. S3 herein for the four dihalogen derivatives that are discussed in the main text.

## 1.4 Frequency Analysis along IRCs

### 1.4.1 Characterization of Transition States and Bifurcations

The analysis of the evolution of vibrational modes in the harmonic approximation along reaction paths allows one to gain additional information about the reaction mechanism. Recent studies used this idea in particular to investigate bifurcations in more detail. [10] In this respect, the vibrational mode belonging to the imaginary frequency of the TS is of special interest. The evolution of the magnitude of the frequency ($y$-axis, imaginary frequencies are represented by the corresponding negative value) that is related to this particular vibrational mode is qualitatively sketched along the reaction path (or IRC) on a PES that is characterized by a normal TS in Fig. S4a. Starting at a positive value in the reactant region, the frequency of

the "soft mode" decreases and reaches a value of zero at the inflection point of the reaction path. From this point on, the normal mode analysis yields a single imaginary frequency. After having passed the TS, the frequency belonging to the unstable vibrational mode at the TS eventually turns positive again.

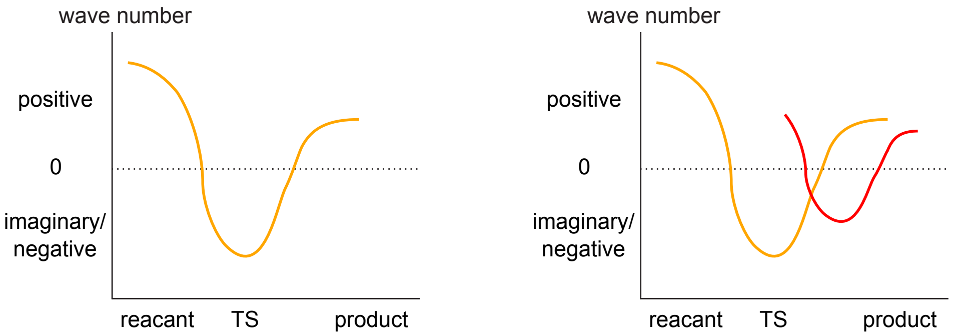


a) PES with a single TS    b) PES with a TS and a downhill bifurcation

Figure S4: Schematic evolution of the lowest frequencies along the reaction paths (as e.g. parameterized using IRCs) on a PES with a single TS in panel (a) and on a PES with a TS and a subsequent downhill bifurcation in (b). The frequency corresponding to the TS is shown using yellow lines whereas that corresponding to the downhill bifurcation is plotted as a red line.

In contrast to scenario (a) where a single product species is generated, Fig. S4b depicts schematically the evolution of the lowest frequencies in the TS region for a PES that possesses a downhill (post-TS) bifurcation, such as the one visualized by Fig. 1(a) in the main text, which leads to two distinct reaction products. The first vibrational mode (yellow line in Fig. S4b) corresponds to the TS and thus features the same trend as found on a PES with only one TS as shown in panel (a). However, before this first frequency turns back to positive values after having passed this TS, a second mode becomes unstable and thus yields imaginary frequencies in some IRC interval on the product (post-TS) side of the pathway. This second imaginary frequency is related to the vibrational mode that directly interconnects the two different product species, which get separated as a result of the bifurcation that occurs after the TS has been surmounted via a second transition state denoted as $T_{1-2}$ in Fig. 1(a) in the main text. The two vibrational modes belonging to these two imaginary frequencies are orthogonal to each other and describe the key atomic displacements along the reaction path. Scenario (b) is relevant for bifurcations as discussed in the main text that decide about both, dis- and conrotatory ring-opening as well as left/right halogen migration which lead in total to four product species that can be obtained from one and the same reactant molecule (see Fig. 2 as well as Fig. 5(d) and (e) in the main text).

### 1.4.2 Force-dependent Frequency Analysis

The analysis described in the previous section can straight-forwardly be extened to our force-transformed PESs to gain further insight into the reaction scenario as discussed in the main text, although frequency analyses have to be interpreted carefully if the analyzed structure is not a stationary point on the PES. For this purpose, the lowest two frequencies along the reaction paths of the *disrotatory* ring-opening reaction of our *trans-g*DCC reactant (*trans*-1,1-dichloro-2,3-dimethylcyclopropane)

at selected constant forces are depicted in the left column of Fig. S5 in the thermal limit (top panel) and finite forces of 1.0 and 1.5 nN (middle and bottom). This scenario, which decides within the disrotatory ring-opening channel about left/right chlorine migration at the corresponding left-right downhill bifurcation, is the one that corresponds to the thermally allowed disrotatory path that is presented in the main text in terms of Fig. 3(b) in the zero force limit. At finite forces but before reaching the topological catastrophe at $F_0^{\mathrm{crit}} \approx 1.6$ nN, the situation is the one that is represented schematically in Fig. 5(d) of the main text *after* the system has committed itself to the disrotatory channel, thus *having passed* the disrotatory-conrotatory uphill bifurcation.

Akin to the purely qualitative discussion in the previous section, the regions corresponding to reactant and product species feature only positive frequencies as required for minima on PESs. In the course of the reaction, however, these frequencies are systematically lowered, which implies a softening of the corresponding mode. At the TS, the PES yields one imaginary frequency (light blue line), as expected for a first-order saddle point. In addition, shortly after the TS toward the product side of the IRCs, a second imaginary frequency (dark blue) occurs in line with the earlier discussed manifestation of post-TS bifurcations in terms of frequency analyses.

A detailed analysis of the two normal modes having the lowest frequencies along the reaction path shows that the frequencies are caused by different quasi-local vibrations. We therefore dissected the modes of the frequency analysis in terms of key displacement components to elucidate the evolution of particular vibrations along the reaction paths and selected the two most relevant ones as shown in the right column of Fig. S5. The responsible vibrational displacements, depicted schematically in Fig. S6, contain the two main motions of the chlorine atom along the reaction path. The first one is essentially a local carbon-chlorine stretching vibration which leads to dissociation of the bond between atom C3 and Cl7 upon its softening (see Fig. 5(c) in the main text or Fig. S1b herein for atom numbering). The second one describes the chlorine bending vibration that decides after softening about left or right migration of the partially dissociated chlorine atom.

Along these disrotatory reaction paths, both in the thermal limit and at small to intermediate forces, the carbon-chlorine stretching vibration (yellow lines in the right column of Fig. S5) sets in first. In the reactant region of the IRC, it assumes a value of approximately $700\,\mathrm{cm}^{-1}$, which is typical for a C–Cl bond [11]. At an RSD of $-0.5\,\text{Å}$, this frequency becomes imaginary for the first time and stays imaginary beyond the TS. Up to this point, the evolution of the frequencies follows the expected behavior of a reaction *via* a single TS but without bifurcation as depicted in Fig. S4a. However, when the reaction proceeds and the frequency of the carbon-chlorine stretching vibration increases again, the chlorine bending vibration softens and becomes imaginary. For a short period along the reaction paths the two vibrations are both imaginary, before the carbon-chlorine stretching vibration becomes positive again. This second imaginary frequency, after having passed the TS, is associated to another TS in close proximity to the former and is a strong indication for a post-TS (downhill) bifurcation. In the present case, the additional TS describes the chlorine left/right migration at the left-right downhill bifurcation and causes the presence of two imaginary frequencies for the disrotatory ring-opening reaction. The underlying PES corresponds topologically to the scenario that is sketched in Fig. 1(a) of the main text.

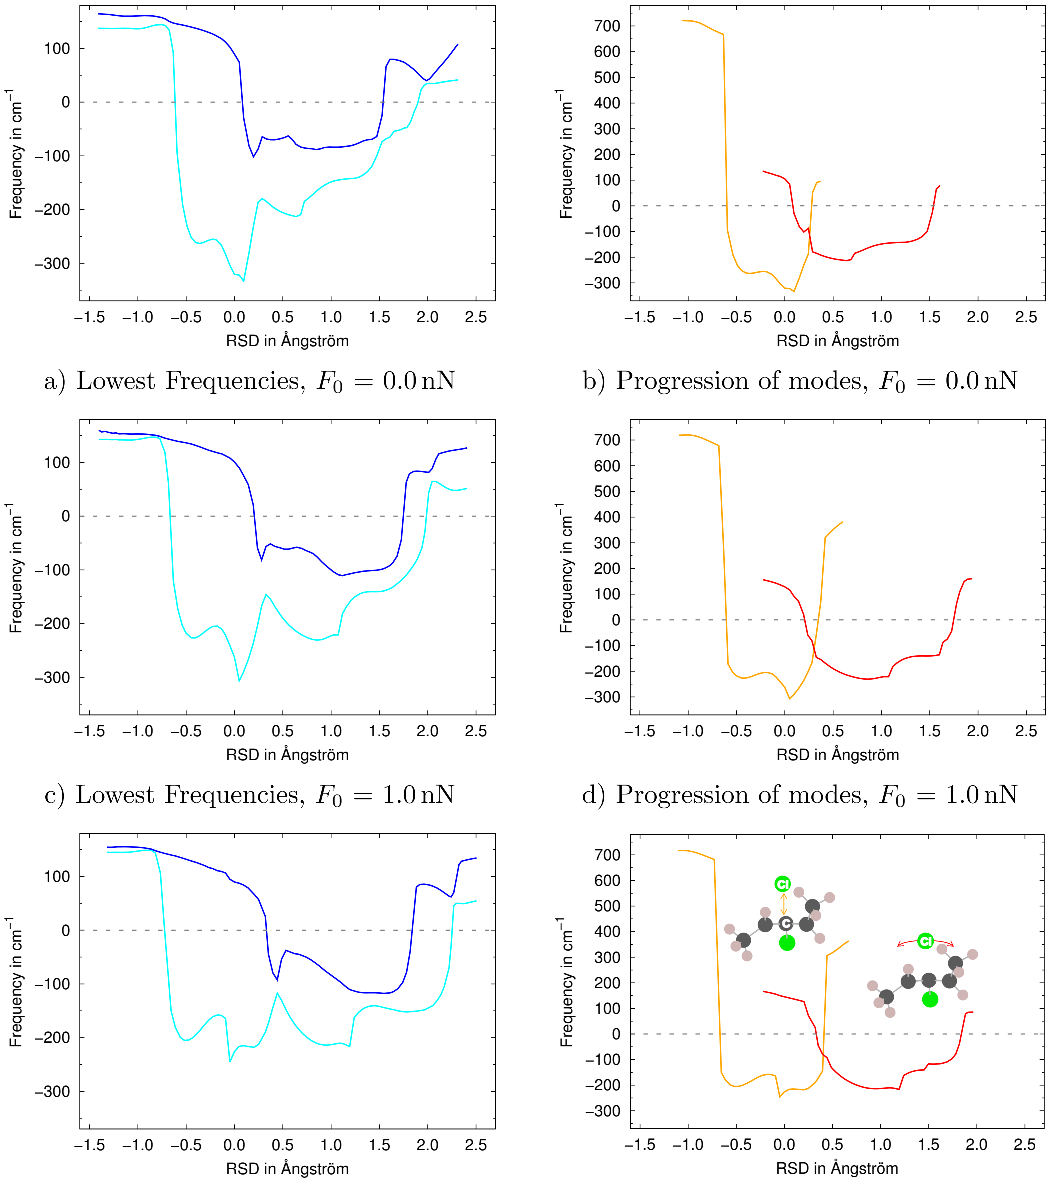


a) Lowest Frequencies, $F_0 = 0.0\,\mathrm{nN}$

b) Progression of modes, $F_0 = 0.0\,\mathrm{nN}$

c) Lowest Frequencies, $F_0 = 1.0\,\mathrm{nN}$

d) Progression of modes, $F_0 = 1.0\,\mathrm{nN}$

e) Lowest Frequencies, $F_0 = 1.5\,\mathrm{nN}$

f) Progression of modes, $F_0 = 1.5\,\mathrm{nN}$

Figure S5: Frequency analysis along the IRCs for disrotatory ring-opening of (2*S*,3*S*)-1,1-dichloro-2,3-dimethylcyclopropane (i.e. *trans*-*g*DCC) in the thermal limit (top panel) and at constant forces below the critical force $F_0^{\mathrm{crit}} \approx 1.6$ nN and thus in the regime of small up to intermediate forces before the topological catastrophe occurs. Left column: Evolution of the lowest (light blue) and second lowest (dark blue) frequencies. Right column: Evolution of the frequencies corresponding to the two relevant vibrational displacements (C-Cl stretching mode (yellow), Cl bending mode (red)) as depicted in the inset of panel (f), see text and also Fig. S6.

## 1.5 Reconstruction of Force-transformed Potential Energy Surfaces

The isotensional *ab initio* molecular dynamics simulations [12] have been conducted as trajectory shooting simulations [1] on the basis of the Car-Parrinello method. [13] Starting at the (optimized) TSs at a variety of constant forces between 0.0 und 3.0 nN, shooting trajectories under the influence of the corresponding constant force

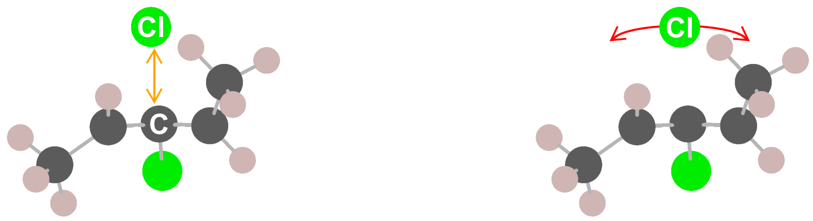


a) C-Cl stretching mode    b) Cl bending mode

Figure S6: Schematic representation of the vibrational displacements that lead to the frequencies as shown in the right column of Fig. S5.

have been generated. The external forces have been applied explicitly on the basis of our EFEI [14] isotensional formalism (see Ref. 15 for similar and alternative approaches) as implemented in our in-house version of the CPMD program suite. [16] Following our earlier work, [1] the open-shell BLYP functional has been used together with pseudopotentials and plane waves up to 100 Ry. In the context of the canonical ensemble (NVT), we have chosen a temperature of 300 K and separate Nosé-Hoover thermostats for ions and orbitals using a time step of 4 a.u. ($\approx$ 0.1 fs) together with a fictitious orbital mass of 400 a.u.. Finite cluster boundary conditions [12] have been imposed in the framework of a plane wave basis using a cubic box with an edge length of 15 Å. With the help of a structural criterion, the propagation of the trajectories has been terminated as soon as they are close to either the reactant or one of the product structures in order to save computer time since only the TS and bifurcation regions are of interest here; this implies that the energy landscape is not that well sampled in the reactant and product wells. The subsequent reconstruction and analysis of the force-transformed potential energy surfaces (FT-PES) was based on already existing trajectories [1] that have been extended by additional such simulations.

The aim of these simulations in the present context was an *a posteriori* reconstruction of the FT-PES as a function of force in a subspace spanned by three collective variables (CVs, see main text or also below) upon using all *ab initio* molecular dynamics simulation trajectories that have been generated at many different forces. The key advantage of this approach is that systematic inclusion of isotensional trajectories generated at a set of distinct force values, ranging from 0 to 3 nN, samples a wide range of differently distorted structures along all kinds of pathways, back to the reactant and forward to the different products, and thus provides a vast data pool of electronic energies depending on molecular configuration which underlies our reconstruction of the FT-PES as a function of a *continuous* force variable. Three CVs have been identified to describe the important parts of the reactions. As the ring-opening and thus the bond breaking of the carbon-carbon bond within the three-membered cyclopropane ring constitutes a major part of the reaction, the corresponding distance C2–C4 distance (see Fig. 5(c) in the main text or Fig. S1 herein for atom numbering) has been chosen as the first variable, CV1. Next, the dihedral angle of what we call the right methyl group is used as CV2 to discriminate between disrotatory and conrotatory trajectories. Last but not least, in order to differentiate between the left and right products, the relative position of the migrating chlorine atom, which is Cl7, is employed as our third dimension, CV3. Therefore, the resulting FT-PES is not represented in the full-dimensional space defined in terms of all

39 internal degrees of freedom, but in a reduced 3D reaction subspace spanned by these 3 CVs, which is why we call it the force-transformed effective potential energy surface (FT-ePES).

The advantage offered by this considerable dimensionality reduction is that a scalar function defined on three-dimensional space can not only easily be visually inspected in order to get qualitative ideas concerning its topology. More importantly, such a landscape can be quantitatively analyzed more readily in terms of its topological features beyond simple stationary points, such as minima and first-order saddle points corresponding to reactant/product states and transition states, respectively. Obviously, getting access to properties such as bifurcations, being in general not stationary points, is of key importance in the present context.

For each and every configuration that has been generated in the set of all trajectories, the three CVs, the corresponding electronic energy, and the mechanical coordinate, i.e. the distance between the carbon atoms of the two methyl groups to which the colinear external force is applied according to Fig. 5(c) in the main text, have been extracted. The three CVs have been used to construct a 3D grid and the electronic energies of all sampled configurations have been assigned to the corresponding grid points. For the reconstructed effective energy landsape at zero force (ePES) the electronic energy with the lowest value has been chosen at each grid point. To arrive at the FT-ePES at finite forces, the additional mechanical work term, being the product of external force and mechanical coordinate in the framework of the EFEI approach, has to be added to the electronic energy. Among these total EFEI energies, the lowest value has been selected at each grid point and has been used to construct the ePES at the desired *continuous* force value. With the help of this procedure, FT-ePESs can be generated as a function of force.

Despite this dramatic reduction of the dimension, even a 3D representation of a complex landscape can be difficult to visualize. Thus, for deeper insights into the nature of the FT-ePESs, 2D slices have been generated as depicted in Figs. 6 and 8 of the main text. To this end, with the help of the program Paraview [17] (Version 3.14.1), we have selected planes in the 3D data at the selected representative forces. For visualization of energy differences we have applied both colors and contour lines. The positioning and orientation of the 2D-slices has been optimized by hand such that the different regions relevant for the ring-opening reaction are covered separately in Figs. 6 and 8 of the main text. Note that the contour lines in the regions of reactant and product minima do not form closed curves as these regions are not exhaustively explored by the shooting trajectories due to applying the structural termination criterion. In addition, the areas of the 2D-slices show a stepped appearance at their borders which results from the finite grid that is used for the reconstruction of the underlying three-dimensional FT-ePES landscapes.

Last but not least, reaction pathways that connect the reactant species to all four products have been mapped using Dijkstra path analysis as explained in the following section in order to fully understand the topology of the FT-ePESs and their force-induced changes.

## 1.6 Dijkstra Path Analysis on Force-transformed Effective Potential Energy Surfaces

### 1.6.1 Method

On the reconstructed FT-ePES, see previous section, we evaluated the reaction pathways that lead from the reactant species via transition states and uphill/downhill bifurcations to the four different products in the following way. First, the lowest points in energy of the respective reactant and product state have been assigned as starting and end point of the path. After that we applied the Dijkstra algorithm [18] to search for paths on the finite 3D grid of energies to connect the reactant with the four products; it is noted in passing that typical path search algorithms as available in standard quantum chemistry packages, which includes IRC procedures, fail to map bifurcations which are usually not stationary points. All adjacent points in energy on our grid are connected by edges. The algorithm assigns weights to these edges based on the energy difference and the distance of the two points. The weights are chosen so that the Dijkstra paths represent a compromise between shortest and steepest path in order to ignore local minima that result from the discrete representation of the FT-ePES that is additionally subject to statistical noise. With this procedure we generated continuous paths on the reconstructed FT-ePES at different forces which continuously connect the reactant to all four products.

The energies along these paths for the thermal limit up to forces of 3 nN are depicted in Fig. S7 for a few selected forces. Being Dijkstra paths, the point of highest energy should not be interpreted as the TS of that path like in static IRC pathways. Thus, the difference of the highest energy along the entire path and the reactant energy is not an activation energy, again in contrast to IRCs. However, the key advantage of the Dijkstra paths over IRCs is that they allow one to extract numerically the topology of the FT-ePES in terms of a specific cascade of transition states and pre- or post-TS bifurcations. Only this information allows one to map out the full reaction pathway from the reactant to a specific product, as depicted in Fig. 5(a) and (b) of the main text, below and above the topological catastrophe, respectively.

### 1.6.2 Results and Discussion

The energies along the Dijkstra paths shown in Fig. S7 for our *trans-g*DCC reactant, (2*S*,3*S*)-1,1-dichloro-2,3-dimethylcyclopropane, feature the following dependence on the magnitude of the external force. In the thermal limit (upper left panel), the four reaction channels share the same path for a while before reaching the bifurcation that decides between the disrotatory (blue) and conrotatory (red) ring-opening process. The separated paths further ascend in energy to reach their respective highest points, which is considerably higher for the conrotatory paths. The resulting energy barrier is thus in favor of the disrotatory ring-opening reaction in the thermal limit, as expected by the Woodward-Hoffmann rules. Importantly, the bifurcation that is disclosed by the Dijkstra path analysis is classified to be an uphill (or pre-TS) bifurcation. After having surmounted their highest points in energy, the emerging dis-left and dis-right as well as the con-left and con-right paths initially share the same pathway, but at a certain point the bifurcation that decides about the direction of the chlorine migration is reached. It is only there that the disrotatory and conrotatory reaction channels split into the respective left and right migration products. In this case, Dijkstra path analysis clearly shows that the left-

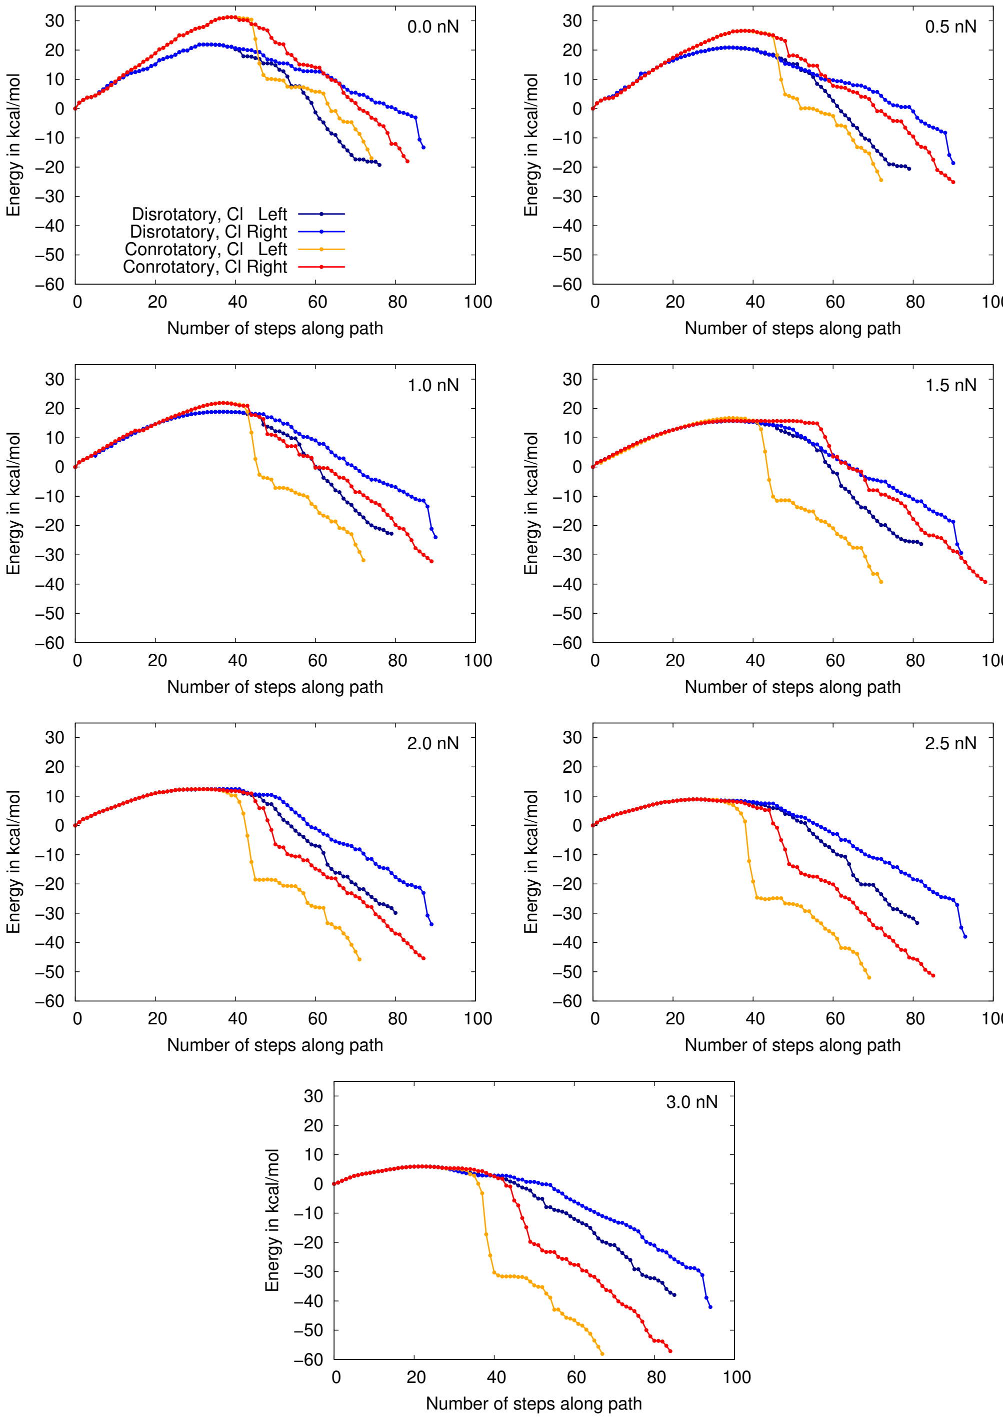


Figure S7: Energy profiles along the Dijkstra paths of (2*S*,3*S*)-1,1-dichloro-2,3-dimethylcyclopropane (i.e. *trans*-*g*DCC) in the thermal limit and at some representative forces relative to the respective energy of the corresponding reactant structure at the same force.

right bifurcation is a downhill (post-TS) bifurcation. This is the scenario that is schematically depicted in panel (d) of Fig. 5 in the main text.

With increasing force, the common part of the path at the beginning of the reaction gets elongated and the uphill bifurcation separating the dis- and conrotatory channel occurs later along the reaction path. For finite forces smaller than the critical force $F_0^{\mathrm{crit}}$, the separation of the dis- and conrotatory paths always appear *before* the highest point in energy is reached along the Dijkstra path. This implies that, before reaching the topological catastrophe, the decision about dis- *versus* conrotatory ring-opening always takes place at a bifurcation on the uphill side along the reaction profile.

At variance with this scenario, forces higher than the critical value $F_0^{\mathrm{crit}}$ cause the common path to be elongated beyond the highest point in energy and consequently all four paths exhibit the same energy barrier. This behavior is already present at 2 nN, but better revealed at 2.5 or 3.0 nN. This implies that the separation of the dis- and conrotatory ring-opening can only happen after the highest point in energy has been surmounted, and thus the corresponding bifurcation is located on the downhill side of the profile followed by two more bifurcations into the left/right migration products. This is the scenario that is schematically depicted in panel (e) of Fig. 5 in the main text.

In conclusion, analyzing carefully the evolution of the energies along the Dijkstra paths according to Fig. S7 supports the description of *trans-g*DCC ring-opening reactions as a function of force that is presented in the main text based on the topology of the energy landscape and its force-induced changes.

### 1.6.3 Comparison to Activation Energies obtained from IRC Analysis

Based on the Dijkstra paths presented in the previous section, energy differences have been calculated as a function of continuous force as the difference between the point of highest energy and the first point on each path that corresponds to the reactant state, recalling that the point of highest energy does *not* correspond to the TS energy for Dijkstra paths. This has been accomplished for both ring-opening mechanisms, i.e. including the conrotatory process down to zero force where it is the Woodward-Hoffmann forbidden reaction, as depicted in Fig. S8a. At zero force, i.e. in the thermal reference case, the energy for the disrotatory reaction is lower in energy than the conrotatory pathway, as expected from the Woodward-Hoffmann rules. With increasing force, the energy differences for both mechanisms decreases as a result of mechanochemical activation. At some critical force, however, the two curves meet each other and the conrotatory mechanism becomes energetically preferred. Thus, the topological catastrophe also decides about the stereochemistry of ring-opening: while the disrotatory process is favored at zero up to intermediate forces, the conrotatory and disrotatory process share the same transition state and therefore feature the same activation energy after the catastrophe happened being the factual basis of the respective discussion in the main text. The same trend as extracted from the present Dijkstra path analysis has been obtained previously based on the usual activation energies, $\Delta E^{\ddagger}$, along the IRCs (see Ref. 2) which is reproduced in Fig. S8b.

Clearly, these energy differences from Dijkstra path analysis must be quantitatively different from activation energies based on IRC analysis for several reasons. First and foremost, IRC paths are constructed in the full-dimensional configuration space, i.e. they are paths on the full dimensional FT-PES, whereas our Dijkstra

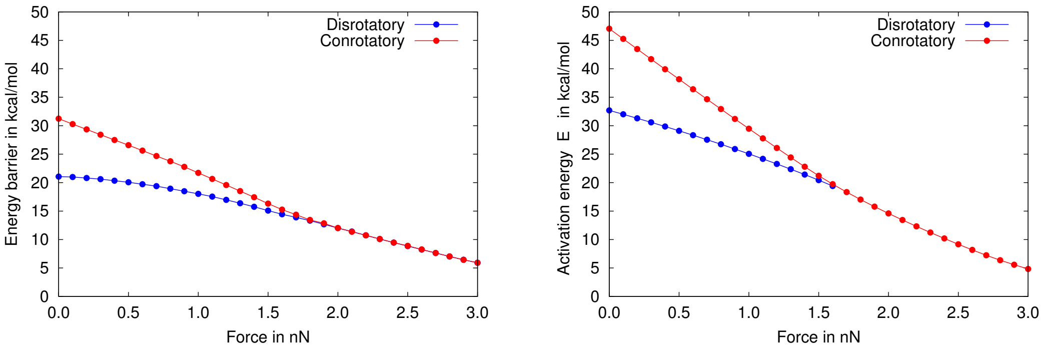


a) Energy difference from the reactant state energy to the highest energy along the Dijkstra paths on the FT-ePES, see text.

b) Total isotensional activation energies including the work term, $\Delta E^{\ddagger}$, obtained from IRC path analysis on the FT-PES.

Figure S8: Energy differences for disrotatory (blue) and conrotatory (red) ring-opening of (2*S*,3*S*)-1,1-dichloro-2,3-dimethylcyclopropane (i.e. *trans*-*g*DCC) as a continuous function of force, see text.

paths have been computed in a specific three-dimensional subspace, FT-ePES, for reasons explained. The Dijkstra paths are thus conceptionally different from IRC paths and, in particular, their highest energies do not correspond to transition states in contrast to IRCs. Next, it must be kept in mind that the underlying FT-ePES has been constructed on a finite 3D grid based on *ab initio* molecular dynamics sampling which introduces numerical noise (as easily seen in Fig. S7). Since the shootings were initiated at transition states, in particular the reactant and product wells are not very well sampled. In addition, although the same electronic structure method (BLYP) has been used, different basis sets have been employed in the dynamical shooting simulations that underly the Dijstra path analysis (namely plane waves up to a cutoff of 100 Ry) and in the static optimizations yielding the IRC paths and energies (namely the TZVP and cc-aug-pVTZ Gaussian basis sets, respectively). Despite these differences, the energy profiles in Fig. S8 obtained from Dijkstra path analysis and straightforwardly from IRCs are astonishingly similar. As explained in the main text, we consider the critical force value, $F_0^{\mathrm{crit}} = 1.6$ nN obtained from IRC analysis to be a reliable estimate for the control parameter at which the topological catastrophe occurs.

## 2 Beyond Cyclopropane Rings

In addition to *trans*-cyclopropanes analyzed in the main text, we also studied ring-opening reactions of other cyclic systems as described in the following. These studies complement the comprehensive analysis of the influence of external forces on the ring-opening reactions of the specific *trans*-cyclopropanes treated in the main text albeit they are *not intended to be exhaustive and systematic* in that respect, and also extend some of our previous work on the mechanochemistry of ring systems [1, 2, 19, 20] using consistently improved methods.

## 2.1 *Cis*-cyclopropane

The methyl groups of the cyclopropane system studied in the main text, see Fig. 5(c) therein or Fig. S1 herein, can also be in the *cis* arrangement, thus being on the same side of the ring, leading to the (2$R$,3$S$)-1,1-dichloro-2,3-dimethylcyclopropane species, i.e. *cis*-1,1-dichloro-2,3-dimethylcyclopropane or *cis*-$g$DCC in short. Similar

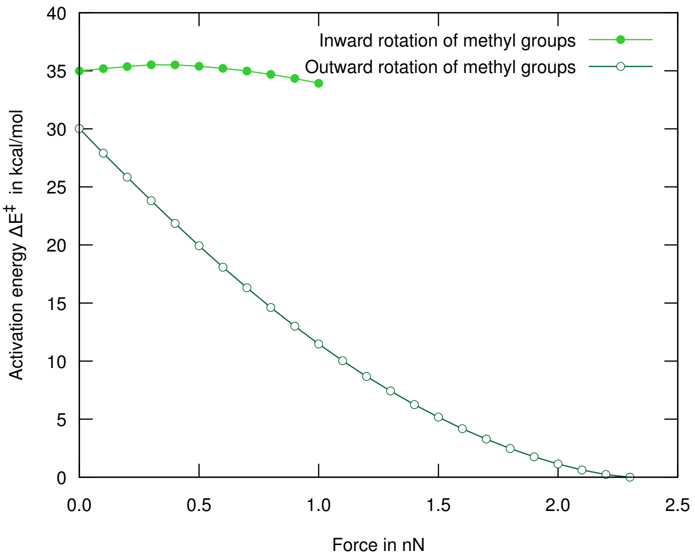


Figure S9: Total isotensional activation energies including the work term, $\Delta E^{\ddagger}$, for (2$R$,3$S$)-1,1-dichloro-2,3-dimethylcyclopropane (i.e. *cis*-$g$DCC) for outward (open dark green circles) and inward (filled light green circles) rotation of the two methyl groups as a function of force.

to the corresponding *trans* stereoisomer, the *cis* system can also undergo a disrotatory ring-opening reaction, where the methyl groups can either rotate inwards or outwards with respect to a reference frame defined similarly as the one in Fig. S1. The corresponding activation energies of these reactions as a function of an external force are shown in Fig. S9. Both reaction pathways are disrotatory processes and, thus, thermally allowed according to the Woodward-Hoffmann rules. Yet, the sterically hindered inward rotation of the methyl groups is energetically disfavored and also rather force-insensitive at all external forces that have been studied. In the thermal limit, this rotation pathway is approximately 5 kcal mol$^{-1}$ higher in energy than its counterpart.

In addition, the two rotation paths show qualitatively different dependences on the external force. The activation energy of the outward rotation is strongly decreasing with increasing external force before it becomes a mechanochemically barrierless process at forces higher than 2.3 nN since the activation barrier is zero at these forces. For outward rotation, the external force acts along the direction of the rotation and therefore strongly promotes the reaction. In stark contrast, in case of the inward rotation, the force acts in the opposite direction and, thus, the associated activation energy is found to be only mildly influenced by the external force. At forces exceeding 1.1 nN no TS could be obtained anymore which is why the corresponding curve in Fig. S9 ends at this value.

The reaction paths of inward and outward rotation also lead to a qualitatively different behavior with respect to the migration of the chlorine atom. While the

inward rotation causes the chlorine atom on the same side of the ring to migrate, in case of outward rotation it is the chlorine atom on the opposite side of the ring that is the leaving group that eventually migrates. This finding is in full accord with expectations based on the De Puy rules [21–23].

In contrast to *trans-g*DCC discussed in the main text, the symmetry-forbidden conrotatory ring-opening in *cis-g*DCC can not be favored by the application of a external tensile forces. Due to the positioning of both methyl groups on the same side of the ring, rotation in the same direction could only be manipulated after fixing the molecule in space, e.g. by attaching it on a surface, and then pulling both methyl group in the same direction.

## 2.2 Cyclobutenes

According to the Woodward-Hoffmann rules, conrotatory ring-opening reactions are favored for cyclobutene systems upon purely thermal activation (i.e. at zero force). In order to eventually favor the symmetry-forbidden disrotatory reaction, the mechanical force needs to be applied to methyl groups that are on the same side of the ring, i.e. in a *cis* arrangement. The symmetry-allowed ring-opening products of two such systems, namely *cis*-3,4-dimethylcyclobutene (*cis*-C4) and *cis*-1,2-dimethylbenzocyclobutene (*cis*-BC4), are depicted in Fig. S10.

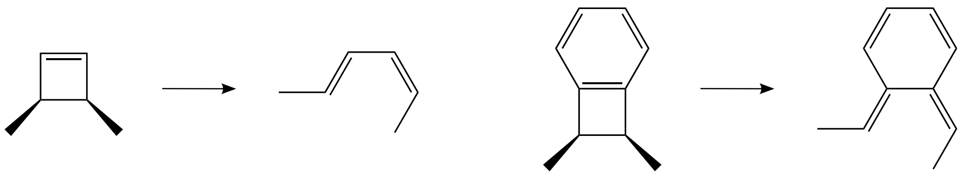

Figure S10: Symmetry-allowed conrotatory ring-opening reaction of *cis*-3,4-dimethylcyclobutene (*cis*-C4) and *cis*-1,2-dimethylbenzocyclobutene (*cis*-BC4) upon thermal activation at zero external force in the left and right panels, respectively.

For *cis*-C4 and *cis*-BC4 the activation energies are depicted in Fig. S11 for both conrotatory and disrotatory ring-opening as a function of constant external force wherever the respective force-transformed TS could be optimized. In the thermal limit at $F_0 = 0$ nN, the conrotatory reaction of *cis*-C4 is favored by approximately 5 kcal mol$^{-1}$ compared to the same process in *cis*-BC4, which is a consequence of the constraints imposed by the flat benzene ring in the latter case. Starting from the thermally allowed TS structures, the mechanical force was increased in small steps in order to optimize the TSs at finite forces, which yields the structure and relative energy of the corresponding force-transformed TS. In this way, we were able to obtain the activation energy of the conrotatory reaction for forces up to 2.0 nN for *cis*-C4. At forces of 2.1 nN, the mechanism of the reaction changes and only the disrotatory TS and thus reaction is observed, which would be the Woodward-Hoffmann forbidden process in the thermal (zero force) limit. Starting from the optimized disrotatory TS at 2.1 nN, the TSs and thus the activation energies have been obtained for the disrotatory process up to 2.8 nN, and also down to 1.7 nN upon slowly releasing the force. At higher forces, we were not able to optimize any longer TS structures, while for smaller forces than 1.7 nN the optimization resulted again in the conrotatory TS; even decreasing the force increments when moving along the force axis did not extend the reported stability limits.

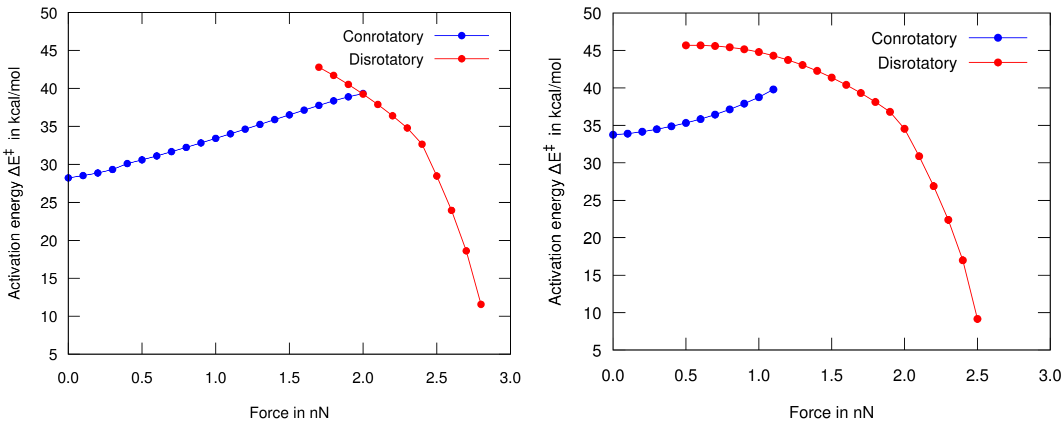


a) *cis*-3,4-dimethylcyclobutene b) *cis*-1,2-dimethylbenzocyclobutene

Figure S11: Total isotensional activation energies including the work term, $\Delta E^{\ddagger}$, for *cis*-C4 (panel a) and *cis*-BC4 (b), see Fig. S10, for conrotatory (blue) and disrotatory (red) ring-opening reactions as a function of force.

In comparison, the larger *cis*-BC4 system has more electronic and structural degrees of freedom due to the attached benzene ring. Starting in the thermal limit, we were able to optimize TSs of the conrotatory reaction up to 1.1 nN by stepwise increasing the external force. At 1.2 nN and beyond, the optimization results in the disrotatory mechanism, being the symmetry-forbidden reaction at $F_0 = 0$ nN. Starting from this structure, we were able to obtain TSs of the disrotatory process for forces between 0.5 and 2.5 nN using the same approach as before. Similar as for *cis*-C4, the mechanism changes back to the conrotatory ring-opening below 0.5 nN and we were not able to obtain disrotatory stationary points with one imaginary frequency in this force regime. Instead, we could only optimize a second-order saddle point at zero force, where the two imaginary frequencies correspond to dis- and conrotatory motion of the two methyl groups. The optimized structure we thereby obtained is comparable to the second-order saddle point described in the literature for cyclobutene. [24–27]

## 2.3 Cyclohexadiene

According to the Woodward-Hoffmann rules, the disrotatory rotation of the substituents is favored for the ring-opening reaction of cyclohexadiene compounds in the absence of external forces. This suggests to investigate the *trans* conformation of the methyl groups in the framework of mechanochemistry, see Fig. S12 for the disrotatory ring-opening of *trans*-5,6-dimethylcyclohexa-1,3-diene (*trans*-C6).

Starting from the disrotatory TS in the thermal limit, we increased the external force stepwise to obtain the TSs on the force-transformed PES as described in the previous sections. In contrast to the smaller ring systems, we did not find the conrotatory TS by stepwise increase of the force. In the entire range from 0 to 3.5 nN, the optimized force-transformed TS structures feature only the disrotratory rotation of the methyl groups as imaginary frequency and the ring-opening conserves this mechanism. However, in a previous mechanochemical study [28] of bare cyclohexa-1,3-diene (i.e. *trans*-C6 without any methyl groups attached) using CASSCF electronic structure, thus including static but neglecting dynamic correlation effects, it was observed that a change of mechanism from disrotatory to conrotatory ring-opening

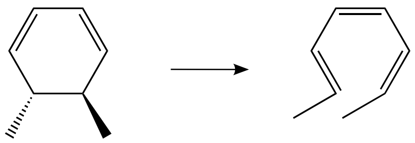

Figure S12: Symmetry-allowed disrotatory ring-opening reaction of *trans*-5,6-dimethylcyclohexa-1,3-diene (*trans*-C6) upon thermal activation at zero external force.

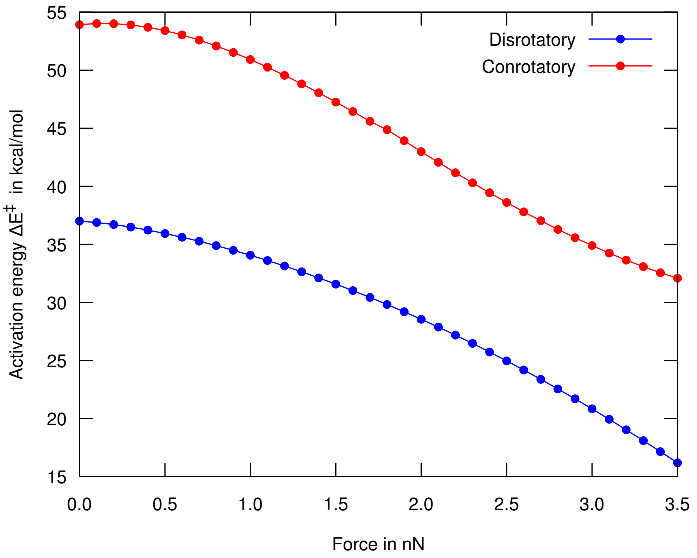


Figure S13: Total isotensional activation energies including the work term, $\Delta E^{\ddagger}$, for *trans*-C6, see Fig. S12, for disrotatory (blue) and conrotatory (red) ring-opening reactions as a function of force.

occurs around 2 nN. As evident from Fig. S13, we were also able to optimize the symmetry-forbidden TS in the thermal limit, and could subsequently optimize the force-transformed conrotatory TS upon applying increasingly large forces. In contrast to the earlier study, [28] our activation energies of the conrotatory process are always larger than those corresponding to disrotatory ring-opening over the whole range of forces, in fact they are found to display a rather similar force dependence. Besides this effect, the external force also influences the reaction paths in the product regime substantially. While in the thermal limit and at small forces the ring-like configuration of the carbon atoms in the non-cyclic product state is sustained, larger forces lead to a stretched structure as one might expect.

## References


[1] P. Dopieralski, J. Ribas-Ariño, D. Marx, *Angew. Chem. Int. Ed.* **2011**, *50*, 7105–7108.

[2] M. Wollenhaupt, M. Krupička, D. Marx, *ChemPhysChem* **2015**, *16*, 1593–1597.

[3] S. J. Getty, D. A. Hrovat, W. T. Borden, *J. Am. Chem. Soc.* **1994**, *116*, 1521–1527.

[4] F. Tian, S. B. Lewis, M. D. Bartberger, W. R. Dolbier, W. T. Borden, *J. Am. Chem. Soc.* **1998**, *120*, 6187–6188.

[5] J. Wang, T. B. Kouznetsova, S. L. Craig, *J. Am. Chem. Soc.* **2016**, *138*, 10410–10412.

[6] J. M. Lenhardt, A. L. Black, S. L. Craig, *J. Am. Chem. Soc.* **2009**, *131*, 10818–10819.

[7] J. Wang, T. B. Kouznetsova, Z. S. Kean, L. Fan, B. D. Mar, T. J. Martínez, S. L. Craig, *J. Am. Chem. Soc.* **2014**, *136*, 15162–15165.

[8] F. Neese, *Wiley Interdiscip. Rev.: Comput. Mol. Sci.* **2012**, *2*, 73–78.

[9] M. J. Frisch, et al., *Gaussian 09 Revision C.01*, Gaussian Inc. Wallingford CT 2009, http://www.gaussian.com.

[10] S. Maeda, Y. Harabuchi, Y. Ono, T. Taketsugu, K. Morokuma, *Int. J. Quantum Chem.* **2015**, *115*, 258–269.

[11] M. Hesse, H. Meier, B. Zeeh, *Spektroskopische Methoden in der organischen Chemie*, Thieme, **2005**.

[12] D. Marx, J. Hutter, *Ab Initio Molecular Dynamics: Basic Theory and Advanced Methods*, Cambridge University Press, **2009**.

[13] R. Car, M. Parrinello, *Phys. Rev. Lett.* **1985**, *55*, 2471–2474.

[14] J. Ribas-Ariño, M. Shiga, D. Marx, *Angew. Chem.* **2009**, *121*, 4254–4257.

[15] J. Ribas-Ariño, D. Marx, *Chem. Rev.* **2012**, *112*, 5412–5487.

[16] J. Hutter, *et al.*, `CPMD` *Program Package,* `http://www.cpmd.org`.

[17] `ParaView` *Program Package.* `http://www.paraview.org`.

[18] E. Dijkstra, *Numer. Math.* **1959**, *1*, 269–271.

[19] J. Ribas-Ariño, M. Shiga, D. Marx, *J. Am. Chem. Soc.* **2010**, *132*, 10609–10614.

[20] P. Dopieralski, P. Anjukandi, M. Rückert, M. Shiga, J. Ribas-Ariño, D. Marx, *J. Mater. Chem.* **2011**, *21*, 8309–8316.

[21] R. Hoffmann, R. B. Woodward, *J. Am. Chem. Soc.* **1965**, *87*, 2046–2048.

[22] R. Hoffmann, R. B. Woodward, *Acc. Chem. Res.* **1968**, *1*, 17–22.

[23] R. B. Woodward, R. Hoffmann, *Angew. Chem. Int. Ed. Engl.* **1969**, *8*, 781–853.

[24] J. Breulet, H. F. Schaefer III, *J. Am. Chem. Soc.* **1984**, *106*, 1221–1226.

[25] J. M. Oliva, J. Gerratt, P. B. Karadakov, D. L. Cooper, *J. Chem. Phys.* **1997**, *107*, 8917–8926.

[26] S. Sakai, *J. Mol. Struct.: Theochem* **1999**, *461-462*, 283–295.

[27] P. S. Lee, S. Sakai, P. Hörstermann, W. R. Roth, E. A. Kallel, K. N. Houk, *J. Am. Chem. Soc.* **2003**, *125*, 5839–5848.

[28] A. Bailey, N. J. Mosey, *J. Chem. Phys.* **2012**, *136*, 044102.
